# Supplementary material for: Fully scalable online-preprocessing algorithm for short oligonucleotide microarray atlases
Source: arXiv:1212.5932 source file (2012-12-27)
Supplement: Supplementary file 1 [file supplement.pdf]

# Fully scalable online-preprocessing algorithm for short oligonucleotide microarray atlases: Supplementary Material

Leo Lahti, Aurora Torrente, Laura L. Elo, Alvis Brazma, and Johan Rung

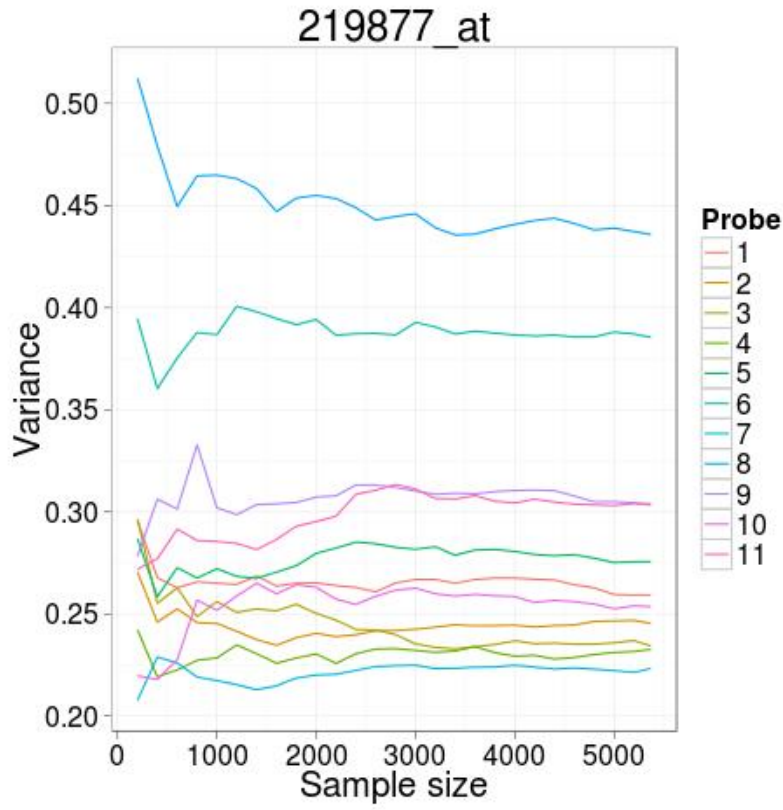

Figure 1: Convergence of probe variance estimates from the Online-RPA algorithm with respect to sample size for the probeset 219877\_at in the Lukk et al. (2010) data set.

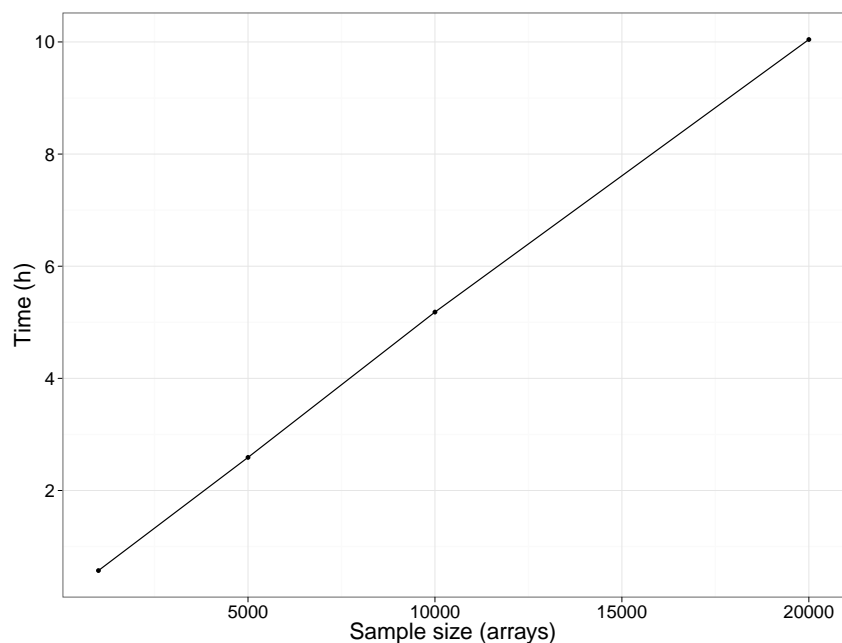

Figure 2: Running time of the Online-RPA preprocessing algorithm scales linearly with respect to sample size. The calculations were performed on a Z400 Desktop with four 3.06 GHz processor cores.

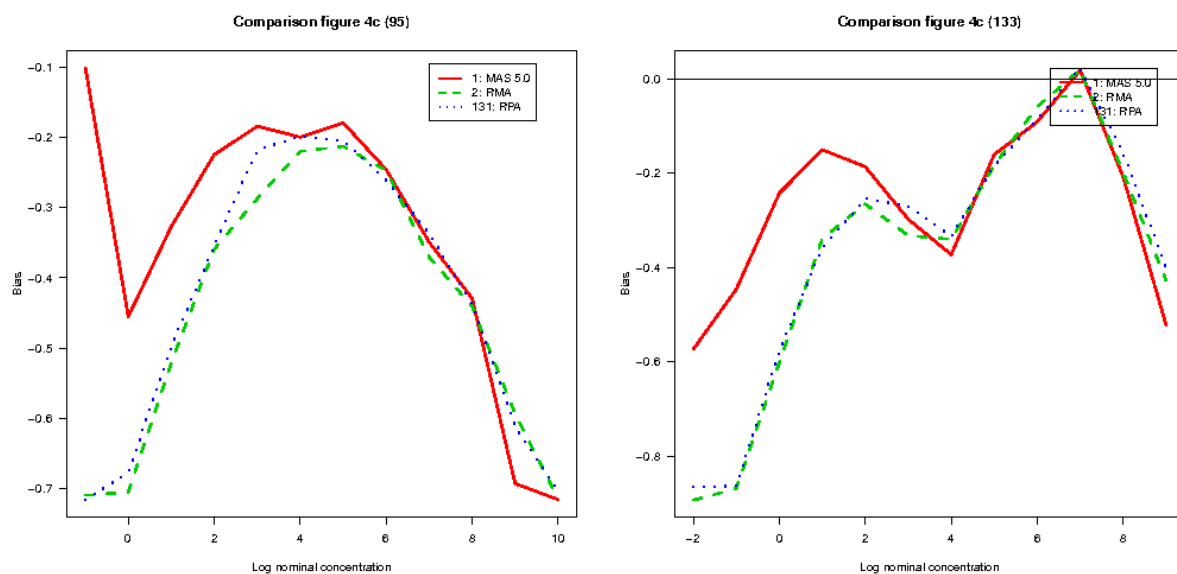

Figure 3: Bias in the AffyCompIII spike-in data sets for MAS5, RMA, and RPA, estimated as the difference between the observed and expected slope for log fold-change as a function of the total nominal concentration. Values close to zero indicate good performance for the algorithm. In this comparison, MAS5 has the lowest overall bias. For further details, see Cope et al., 2004.

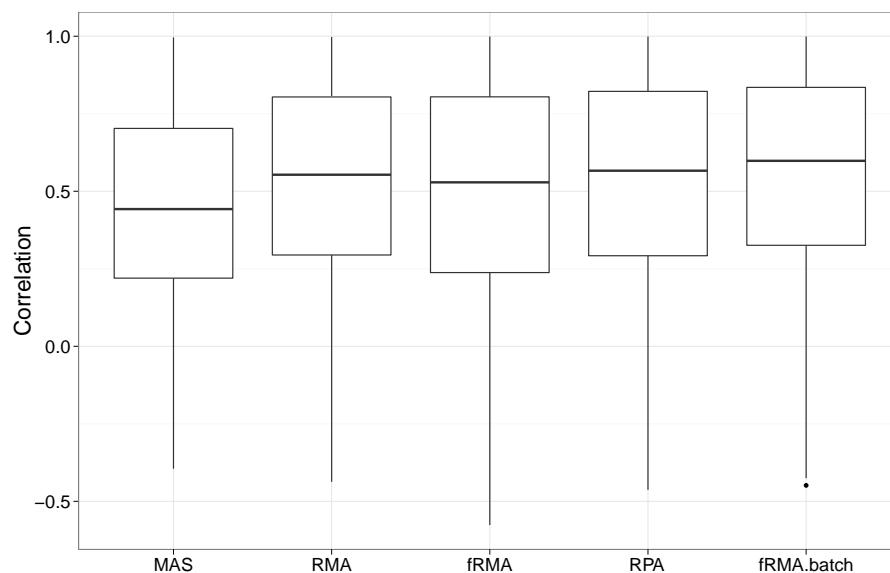

Figure 4: Pearson correlation was calculated for each Affymetrix probeset pair sharing the same EnsemblID (Bioconductor hgu133a.db package). The average correlation over all pairs: MAS5 0.46, RMA 0.53, fRMA 0.51, fRMA.batch 0.55 and RPA 0.54. The differences between the preprocessing methods were statistically significant (paired Wilcoxon test P-value  $< 0.01$ ). In this comparison, RPA performs better than MAS5, RMA and fRMA.
